# Supplementary material for: Towards Carbon Footprint-Aware Recommender Systems for Greener Item Recommendation
Source: arXiv:2503.17201 source file (2025-03-21)
Supplement: Supplementary file 1 [file Appendix_converstion.tex]

\section{Conversion of Ingredient Weights} \label{app:conv}

Table~\ref{tab:my-table-conv} provides the conversion rates of non-standard quantity measures to grams. In addition, the "pinch" metric was typically used for spices and salt and we choose salt as the representative ingredient with a conversion rate of 0.36 grams.

\definecolor{Gray}{gray}{0.9}
\begin{table}[H]
\caption{Categories, their representations, as well as their corresponding weights conversion from pint, cup, teaspoon, and tablespoon to grams. "na." implies that measuring approach was not present for the specific category. }
\label{tab:my-table-conv}
\begin{tabular}{lccccc}
\hline\hline
\rowcolor{Gray}
{\textbf{Category}}     & \textbf{Represented by} & \textbf{Pint-to-g} & \textbf{Cup-to-g} & \textbf{Teaspoon-to-g} & \textbf{Tablespoon-to-g} \\
{liquids}               & water                   & 473.18   & 236.59   & 4.93 & 14.79         \\
\rowcolor{Gray}
{sugars and sweeteners} & raw sugar               & 414.02   & 227.36  & 4.74  & 14.21        \\
{flours}                & all-purpose flower      & 250.31   & 125.16 & 2.61 & 7.82         \\
\rowcolor{Gray}
{oils and fats}         & olive oil               & 434.38    & 217.66   & 4.53  & 13.6       \\
{spices}                & cinnamon                & 264.98   & 132.49  & 2.76  & 8.28         \\
\rowcolor{Gray}
{nuts}                  & almonds                 & 217.66     & 108.83  & na.  & na.       \\
{fruits and vegetables} & onion                   & 104.10  & 150    & na.  &na.      \\
\hline\hline
\end{tabular}
\end{table}
